# Supplementary material for: Asymptotics of feature learning in two-layer networks after one gradient-step
Source: arXiv:2402.04980 source file (2024-06-04)
Supplement: Supplementary file 1 [file details_numerics.tex]

\section{Details on the numerics}
\label{sec:app:details_numerics}
\dots
